# Supplementary material for: Near-Optimal No-Regret Learning for Correlated Equilibria in Multi-Player General-Sum Games
Source: arXiv:2111.06008 source file (2023-01-24)
Supplement: Supplementary file 1 [file appendix_arbo.tex]

\section{An Illustrative Example of Arborescences}
\label{section:example}

To further clarify \Cref{definition:directed_tree}, in \Cref{fig:directed_trees} we illustrate the set of all directed trees with $4$ nodes and a fixed root at node $1$.

\begin{figure}[ht]
    \centering\input{figs/arborescences}
    \caption{Set $\treeset[1]^4$ of all directed trees rooted at node $1$ in a graph with $4$ nodes.}
    \label{fig:directed_trees}
\end{figure}
